# Supplementary material for: How Do Large Language Models Understand Graph Patterns? A Benchmark for Graph Pattern Comprehension
Source: arXiv:2410.05298 source file (2025-04-20)
Supplement: Supplementary file 1 [file 03_topology-based.tex]

\section{topology-based patterns}
%\subsection{Results of topology-based pattern detection}
\input{Tables/topology_pattern_detection_whole}
